# Supplementary material for: Simon's model does not produce Zipf's law: The fundamental rich-get-richer mechanism for any power-law size ranking
Source: arXiv:2604.13184 source file (2026-04-14)
Supplement: Supplementary file 1 [file rich-get-richer-complete.supplementary.tex]

%% using appendix files
